# Supplementary material for: Sequential Kalman filter for fast online changepoint detection in longitudinal health records
Source: arXiv:2310.18611 ancillary file (2024-01-01)
Supplement: Supplementary file 1 [file SKFCPD_supplement.pdf]

# Supplementary materials of Sequential Kalman Filter of Fast Online Changepoint Detection for Correlated Data

## S1 Temporal Correlations in COVID-19 Patient Data

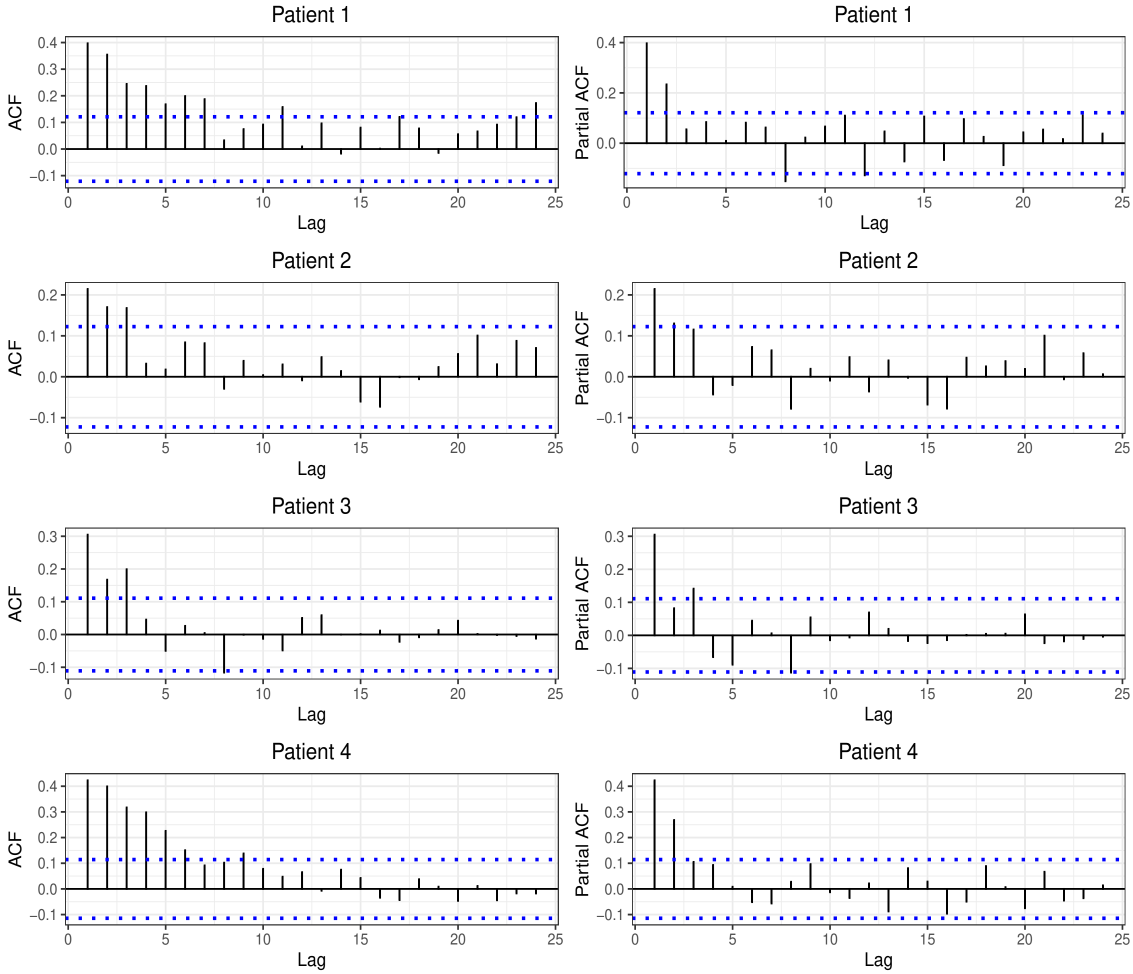


Figure S1: ACF and partial ACF for the predictive probability sequences of four dialysis patients in Section 1.

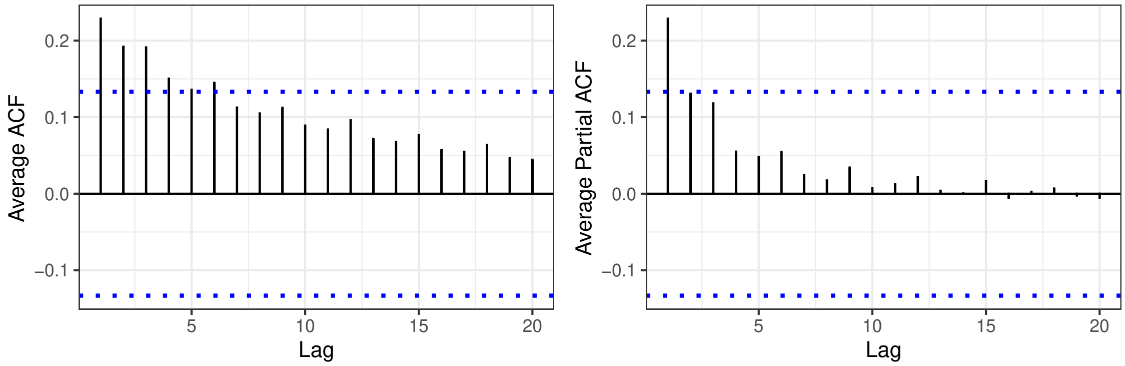


Figure S2: Average ACF and Partial ACF for the predictive probability sequences of all dialysis patients.

Figure S1 shows autocorrelation function (ACF) and partial ACF (Box et al., 2015) in the probability sequences of four COVID-19 patients, and the averages among all patients are shown in Figure S2. We found that positive lag temporal correlations are common in longitudinal measurements of dialysis patients. The temporal correlation is modeled in SKF, enabling detection of the changepoint more quickly and precisely than other methods, such as BOCPD and CUSUM as shown in Table 1.

# S2 Derivation of Equation (1)

We show the derivation of Equation (1) for BOCPD. At the $n$th time point, the joint distribution of measurements and most recent changepoint $C_n$ can be derived below

$$
\begin{aligned}
& p\left(\mathbf{y}_{1:n}, C_n = t_i\right) \\
=& \sum_{j=1}^{n-1} p\left(\mathbf{y}_{1:n}, C_n = t_i, C_{n-1} = t_j\right) \\
=& \sum_{j=1}^{n-1} p(y_n, C_n = t_i \mid \mathbf{y}_{1:(n-1)}, C_{n-1} = t_j) p(\mathbf{y}_{1:(n-1)}, C_{n-1} = t_j) \\
=& \sum_{j=1}^{n-1} p(y_n \mid \mathbf{y}_{1:(n-1)}, C_{n-1} = t_j, C_n = t_i) p(C_n = t_i \mid C_{n-1} = t_j, \mathbf{y}_{1:(n-1)}) p(\mathbf{y}_{1:(n-1)}, C_{n-1} = t_j) \\
=& \underbrace{p\left(y_n \mid \mathbf{y}_{i:(n-1)}, C_n = t_i\right)}_{\text{predictive distribution}} \sum_{j=1}^{n-1} \underbrace{p\left(C_n = t_i \mid C_{n-1} = t_j\right)}_{\text{hazard}} p\left(\mathbf{y}_{1:(n-1)}, C_{n-1} = t_j\right) \\
=& \begin{cases} p\left(y_n \mid \mathbf{y}_{i:(n-1)}, C_n = t_i\right) \left(1 - H(t_i)\right) p\left(\mathbf{y}_{1:(n-1)}, C_{n-1} = t_i\right), & i < n, \\ p\left(y_n \mid C_n = t_n\right) H(t_n) \sum_{j=1}^{n-1} p\left(\mathbf{y}_{1:(n-1)}, C_{n-1} = t_j\right), & i = n, \end{cases}
\end{aligned}
$$

where the first three equations directly follow from the conditional probability equation. The fourth equation is based on Assumptions 1 and 2. First, given the most recent changepoint $C_n = t_i$, the observations before and after time $t_i$ are independent. i.e., $(\mathbf{y}_{1:i-1} \perp\!\!\!\perp \mathbf{y}_{i:n}) \mid C_n = t_i$. This leads to the expression $p(y_n \mid \mathbf{y}_{1:(n-1)}, C_{n-1} = t_j, C_n =$

$t_i) = p(y_n \mid \mathbf{y}_{i:(n-1)}, C_n = t_i)$. Second, the time point of the most recent changepoint at the $n$th time $C_n$, conditioned on the most recent changepoint at the $(n-1)$th time $C_{n-1}$, is independent of the previous observations $\mathbf{y}_{1:(n-1)}$, resulting in the expression $p(C_n = t_i \mid C_{n-1} = t_j, \mathbf{y}_{1:(n-1)}) = p(C_n = t_i \mid C_{n-1} = t_j)$.

Two scenarios are considered in the last equation. First, when $i < n$, the most recent changepoint $C_n = t_i$ is prior to time $t_n$, indicating that time $t_n$ is not a changepoint. By the definition of hazard function in Section 2.1, the summation over $j$ from 1 to $n-1$ in the fourth equation is reduced to $j = i$ in the fifth equation when $i < n$. Second, when $i = n$, meaning that $t_n$ is a changepoint, $C_{n-1} = t_j$ could take any values from $t_1$ to $t_{n-1}$. Consequently, the summation over $p(\mathbf{y}_{1:(n-1)}, C_{n-1} = t_j)$ in the fourth equation still holds in the fifth equation when $i = n$.

# S3 Connections between the Dynamic Linear Model and Gaussian Process Model having a Matérn Covariance with Roughness Parameter being 2.5

We show the connections between the dynamic linear model (DLM) and Gaussian process (GP) model having a Matérn covariance with the roughness parameter being 2.5. For any inputs $(t_i, \dots, t_n) \in \mathbb{R}^{n'}$, where $t_i = C_n$ is the most recent changepoint before time $t_n$, a GP model having the Matérn correlation with the roughness parameter being 2.5 is defined as

$$\left((y(t_i), \dots, y(t_n))^T\right) \mid \mu, \sigma^2, \mathbf{R}_{n'}, \sigma_0^2 \sim \mathcal{MN}(\mu \mathbf{1}_{n'}, \sigma^2 \mathbf{R}_{n'} + \sigma_0^2 \mathbf{I}_{n'}), \tag{S1}$$

where $n' = n - i + 1$ is the number of observations from time $t_i$ to $t_n$ and $\mathbf{R}_{n'}$ is a $n' \times n'$ matrix with the covariance function

$$c(t, t') = \left(1 + \frac{\sqrt{5}d}{\gamma} + \frac{5d^2}{3\gamma^2}\right) \exp\left(-\frac{\sqrt{5}d}{\gamma}\right), \tag{S2}$$

where $d = |t - t'|$ and $\gamma$ is the range parameter. Denote $\lambda = \frac{\sqrt{5}}{\gamma}$ and $d_{i,k} = |t_{i+k-1} - t'_{i+k-1}|$ for $k = 1, \dots, n'$. For simplicity, we denote $y_{i+k-1} = y(t_{i+k-1})$, the observation at time $t_{i+k-1}$, which does not need to be equally spaced. The DLM is defined as follows.

$$\begin{aligned} y_{i+k-1} &= \mu + \mathbf{F}_{i,k} \boldsymbol{\theta}_{i,k} + \epsilon_k, \quad \epsilon_k \sim \mathcal{N}\left(0, \sigma_0^2\right), \\ \boldsymbol{\theta}_{i,k} &= \mathbf{G}_{i,k} \boldsymbol{\theta}_{i,k-1} + \mathbf{w}_{i,k}, \quad \mathbf{w}_{i,k} \sim \mathcal{MN}\left(0, \mathbf{W}_{i,k}\right), \end{aligned} \tag{S3}$$

where $\boldsymbol{\theta}_{i,k}$ is a $q$-dimensional latent state process with the initial state $\boldsymbol{\theta}_{i,0} \sim \mathcal{N}(0, \mathbf{B}_0)$, $\mathbf{F}_{i,k}$ is a $1 \times q$ vector, $\mathbf{B}_0$, $\mathbf{G}_{i,k}$ and $\mathbf{w}_{i,k}$ are $q \times q$ matrices, for $k = 1, \dots, n'$. Shown in Hartikainen and Särkkä (2010) and Gu and Xu (2020), the DLM in Equation (S3) is

equivalent to the GP model defined in Equations (S1) and (S2), where

$$
\begin{aligned}
\mathbf{F}_{i,k} &= \begin{bmatrix} 1 & 0 & 0 \end{bmatrix}, \\
\mathbf{G}_{i,k} &= e^{-\frac{\lambda d_{i,k}}{2}} \begin{bmatrix} \lambda^2 d_{i,k}^2 + 2\lambda + 2 & 2\lambda d_{i,k}^2 + 2d_{i,k} & d_{i,k}^2 \\ -\lambda^3 d_{i,k}^2 & -2(\lambda^2 d_{i,k}^2 - \lambda d_{i,k} - 1) & 2 - \lambda d_{i,k}^2 \\ \lambda^4 d_{i,k}^2 - 2\lambda^3 d_{i,k} & 2(\lambda^3 d_{i,k}^2 - 3\lambda^2 d_{i,k}) & \lambda^2 d_{i,k}^2 - 4\lambda d_{i,k} + 2 \end{bmatrix}, \\
\mathbf{W}_{i,k} &= \frac{4\sigma^2\lambda^5}{3} \begin{bmatrix} W_{1,1}^{(i,k)} & W_{1,2}^{(i,k)} & W_{1,3}^{(i,k)} \\ W_{2,1}^{(i,k)} & W_{2,2}^{(i,k)} & W_{2,3}^{(i,k)} \\ W_{3,1}^{(i,k)} & W_{3,2}^{(i,k)} & W_{3,3}^{(i,k)} \end{bmatrix},
\end{aligned}
\tag{S4}
$$

with

$$
\begin{aligned}
W_{1,1}^{(i,k)} &= \frac{e^{-2\lambda d_{i,k}}(3 + 6\lambda d_{i,k} + 6\lambda^2 d_{i,k}^2 + 4\lambda^3 d_{i,k}^3 + 2\lambda^4 d_{i,k}^4) - 3}{-4\lambda^5}, \\
W_{1,2}^{(i,k)} = W_{2,1}^{(i,k)} &= \frac{e^{-2\lambda d_{i,k}}}{2}, \\
W_{1,3}^{(i,k)} = W_{3,1}^{(i,k)} &= \frac{e^{-2\lambda d_{i,k}}(1 + 2\lambda d_{i,k} + 2\lambda^2 d_{i,k}^2 + 4\lambda^3 d_{i,k}^3 - 2\lambda^4 d_{i,k}^4) - 1}{4\lambda^3}, \\
W_{2,2}^{(i,k)} &= \frac{e^{-2\lambda d_{i,k}}(1 + 2\lambda d_{i,k} + 2\lambda^2 d_{i,k}^2 - 4\lambda^3 d_{i,k}^3 + 2\lambda^4 d_{i,k}^4) - 1}{-4\lambda^3}, \\
W_{2,3}^{(i,k)} = W_{3,2}^{(i,k)} &= \frac{e^{-2\lambda d_{i,k}} d_{i,k}^2 (4 - 4\lambda d_{i,k} + \lambda^2 d_{i,k}^2)}{2}, \\
W_{3,3}^{(i,k)} &= \frac{e^{-2\lambda d_{i,k}}(-3 + 10\lambda d_{i,k} - 22\lambda^2 d_{i,k}^2 + 12\lambda^3 d_{i,k}^3 - 2\lambda^4 d_{i,k}^4) + 3}{4\lambda}, \text{ and}
\end{aligned}
\tag{S5}
$$

$$
\mathbf{B}_0 = \begin{bmatrix} \sigma^2 & 0 & -\sigma^2\lambda^2/3 \\ 0 & \sigma^2\lambda^2/3 & 0 \\ -\sigma^2\lambda^2/3 & 0 & \sigma^2\lambda^4 \end{bmatrix}.
$$

# S4 Derivation of Equation (7)

We show the derivation of Equation (7). Denote the observations from times $t_i$ to $t_n$ as $\mathbf{y}_{i:n} = (y_i, \ldots, y_n)^T$. $n' = n - i + 1$ represents the total number of observations from $t_i$ to $t_n$. We assume that all observations in $\mathbf{y}_{i:n}$ are from the same time segment and follow the GP model with the same mean parameter $\mu$ and variance parameter $\sigma^2$. Denote the parameter set as $\mathbf{\Theta} = (\mu, \sigma^2, \gamma, \eta)$. Given an objective prior for $\mu$ and $\sigma^2$ such that $\pi(\mu, \sigma^2) \propto \frac{1}{\sigma^2}$, the likelihood function for $\mathbf{y}_{i:n}$, with $\mu$ and $\sigma^2$ integrated out, has the following form for any

$i < n-1$.

$$
\begin{aligned}
p(\mathbf{y}_{i:n} \mid \gamma, \eta) &= \int p\left(\mathbf{y}_{i:n} \mid \boldsymbol{\Theta}\right) \pi(\mu, \sigma^2) d\mu d\sigma^2 \\
&\propto (2\pi)^{-\frac{n'}{2}} |\mathbf{K}_{n'}|^{-\frac{1}{2}} \\
&\quad \times \int \left(\sigma^2\right)^{-\frac{n'}{2}-1} \exp\left(-\frac{1}{2\sigma^2}(\mathbf{y}_{i:n} - \mu\mathbf{1}_{n'})^T \mathbf{K}_{n'}^{-1}(\mathbf{y}_{i:n} - \mu\mathbf{1}_{n'})\right) d\mu d\sigma^2 \\
&\propto (2\pi)^{-\frac{n'}{2}} |\mathbf{K}_{n'}|^{-\frac{1}{2}} \int \left(\sigma^2\right)^{-\frac{n'}{2}-1} \exp\left(-\frac{1}{2\sigma^2}\mathbf{y}_{i:n}^T \mathbf{M}_{n'} \mathbf{y}_{i:n}\right) \\
&\quad \times \exp\Bigg( - \frac{1}{2\sigma^2} \left(\mu - \left(\mathbf{1}_{n'}^T \mathbf{K}_{n'}^{-1} \mathbf{1}_{n'}\right)^{-1} \mathbf{1}_{n'}^T \mathbf{K}_{n'}^{-1} \mathbf{y}_{i:n}\right)^T \mathbf{1}_{n'}^T \mathbf{K}_{n'}^{-1} \mathbf{1}_{n'} \\
&\quad \times \left(\mu - \left(\mathbf{1}_{n'}^T \mathbf{K}_{n'}^{-1} \mathbf{1}_{n'}\right)^{-1} \mathbf{1}_{n'}^T \mathbf{K}_{n'}^{-1} \mathbf{y}_{i:n}\right) \Bigg) d\mu d\sigma^2 \\
&\propto (2\pi)^{-\frac{n'-1}{2}} |\mathbf{K}_{n'}|^{-\frac{1}{2}} \left(\mathbf{1}_{n'}^T \mathbf{K}_{n'}^{-1} \mathbf{1}_{n'}\right)^{-\frac{1}{2}} \\
&\quad \times \int \left(\sigma^2\right)^{-\frac{n'-1}{2}-1} \exp\left(-\frac{1}{2\sigma^2}\mathbf{y}_{i:n}^T \mathbf{M}_{n'} \mathbf{y}_{i:n}\right) d\sigma^2 \\
&\propto \left(\frac{\pi}{2}\right)^{-\frac{n'-1}{2}} \tau\left(\frac{n'-1}{2}\right) |\mathbf{K}_{n'}|^{-\frac{1}{2}} \left(\mathbf{1}_{n'}^T \mathbf{K}_{n'}^{-1} \mathbf{1}_{n'}\right)^{-\frac{1}{2}} \left(\mathbf{y}_{i:n}^T \mathbf{M}_{n'} \mathbf{y}_{i:n}\right)^{-\frac{n'-1}{2}}, \qquad \text{(S6)}
\end{aligned}
$$

where

$$\mathbf{M}_{n'} = \mathbf{K}_{n'}^{-1} - \mathbf{K}_{n'}^{-1}\mathbf{1}_{n'}\left(\mathbf{1}_{n'}^T \mathbf{K}_{n'}^{-1} \mathbf{1}_{n'}\right)^{-1} \mathbf{1}_{n'}^T \mathbf{K}_{n'}^{-1}.$$

Therefore, for any $i < n-1$, given the likelihood function for $\mathbf{y}_{i:n}$ in Equation (S6), the predictive distribution of $y_n$ given $\mathbf{y}_{i:(n-1)}$ can be derived as follows.

$$
\begin{aligned}
p(y_n \mid \mathbf{y}_{i:(n-1)}, \gamma, \eta) &= \frac{p(\mathbf{y}_{i:n} \mid \gamma, \eta)}{p(\mathbf{y}_{i:(n-1)} \mid \gamma, \eta)} \\
&\propto \frac{\Gamma\left(\frac{n'-1}{2}\right)}{\Gamma\left(\frac{n'-2}{2}\right)} \left(\frac{|\mathbf{K}_{n'}|}{|\mathbf{K}_{n'-1}|}\right)^{-1/2} \left(\frac{\left|\mathbf{1}_{n'}^T \mathbf{K}_{n'}^{-1} \mathbf{1}_{n'}\right|}{\left|\mathbf{1}_{n'-1}^T \mathbf{K}_{n'-1}^{-1} \mathbf{1}_{n'-1}\right|}\right)^{-1/2} \exp\left(-S_{n'}^2\right) \qquad \text{(S7)}
\end{aligned}
$$

where $S_{n'}^2 = \left(\frac{n'-1}{2}\right) \log\left(\mathbf{y}_{i:n}^T \mathbf{M}_{n'} \mathbf{y}_{i:n}\right) - \left(\frac{n'-2}{2}\right) \log\left(\mathbf{y}_{i:(n-1)}^T \mathbf{M}_{n'-1} \mathbf{y}_{i:(n-1)}\right)$.

However, when $i = n-1$, the predictive distribution of $y_n$ given $y_{n-1}$ can't be computed by Equation (S7).This is due to the fact that $n'$, representing the number of observations between time $t_i$ and $t_n$, is equal to 2, which results in the divergent Gamma function $\Gamma(\frac{n'-2}{2}) = \Gamma(0)$. In this case, we need to separately integrate out the parameters $\mu$ and $\sigma^2$ in order to compute the predictive distribution $p(y_n \mid y_{n-1}, \gamma, \eta)$. First, we integrate out $\mu$

with prior distribution $\pi(\mu) \propto 1$ in the joint distribution follows

$$
\begin{aligned}
p(\mathbf{y}_{i:n} \mid \sigma^2, \gamma, \eta) &= \int p\left(\mathbf{y}_{i:n} \mid \boldsymbol{\Theta}\right) \pi(\mu) d\mu \\
&\propto (2\pi)^{-\frac{n'}{2}} |\mathbf{K}_{n'}|^{-\frac{1}{2}} \\
&\quad \times \int \left(\sigma^2\right)^{-\frac{n'}{2}} \exp\left(-\frac{1}{2\sigma^2}(\mathbf{y}_{i:n} - \mu\mathbf{1}_{n'})^T \mathbf{K}_{n'}^{-1}(\mathbf{y}_{i:n} - \mu\mathbf{1}_{n'})\right) d\mu \\
&\propto (2\pi)^{-\frac{n'}{2}} |\mathbf{K}_{n'}|^{-\frac{1}{2}} \int \left(\sigma^2\right)^{-\frac{n'}{2}} \exp\left(-\frac{1}{2\sigma^2}\mathbf{y}_{i:n}^T \mathbf{M}_{n'} \mathbf{y}_{i:n}\right) \\
&\quad \times \exp\Bigg( -\frac{1}{2\sigma^2}\left(\mu - \left(\mathbf{1}_{n'}^T \mathbf{K}_{n'}^{-1} \mathbf{1}_{n'}\right)^{-1} \mathbf{1}_{n'}^T \mathbf{K}_{n'}^{-1} \mathbf{y}_{i:n}\right)^T \mathbf{1}_{n'}^T \mathbf{K}_{n'}^{-1} \mathbf{1}_{n'} \\
&\quad \times \left(\mu - \left(\mathbf{1}_{n'}^T \mathbf{K}_{n'}^{-1} \mathbf{1}_{n'}\right)^{-1} \mathbf{1}_{n'}^T \mathbf{K}_{n'}^{-1} \mathbf{y}_{i:n}\right) \Bigg) d\mu \\
&\propto \left(2\pi\sigma^2\right)^{-\frac{n'-1}{2}} |\mathbf{K}_{n'}|^{-\frac{1}{2}} \left(\mathbf{1}_{n'}^T \mathbf{K}_{n'}^{-1} \mathbf{1}_{n'}\right)^{-\frac{1}{2}} \exp\left(-\frac{1}{2\sigma^2}\mathbf{y}_{i:n}^T \mathbf{M}_{n'} \mathbf{y}_{i:n}\right).
\end{aligned} \tag{S8}
$$

And the predictive distribution, when $i = n-1$, after integrating out $\mu$, is as follows.

$$
\begin{aligned}
&p(y_n \mid \mathbf{y}_{i:(n-1)}, \sigma^2, \gamma, \eta) = p(y_n \mid y_{n-1}, \sigma^2, \gamma, \eta) = \frac{p(\mathbf{y}_{(n-1):n} \mid \sigma^2, \gamma, \eta)}{p(y_{n-1} \mid \sigma^2, \gamma, \eta)}. \\
&\propto \left(\sigma^2\right)^{-\frac{1}{2}} \left(\frac{|\mathbf{K}_{n'}|}{|\mathbf{K}_{n'-1}|}\right)^{-1/2} \left(\frac{\left|\mathbf{1}_{n'}^T \mathbf{K}_{n'}^{-1} \mathbf{1}_{n'}\right|}{\left|\mathbf{1}_{n'-1}^T \mathbf{K}_{n'-1}^{-1} \mathbf{1}_{n'-1}\right|}\right)^{-1/2} \exp\left(-\frac{1}{2\sigma^2}\mathbf{y}_{i:n}^T \mathbf{M}_{n'} \mathbf{y}_{i:n}\right)
\end{aligned}
$$

Then, we integrate out the parameter $\sigma^2$ with the prior distribution $\pi(\sigma^2) \propto \frac{1}{\sigma^2}$.

$$
\begin{aligned}
p(y_n \mid y_{n-1}, \gamma, \eta) &= \int p(y_n \mid y_{n-1}, \sigma^2, \gamma, \eta) \pi(\sigma^2) d\sigma^2 \\
&\propto \int \left(\sigma^2\right)^{-3/2} \left(\frac{|\mathbf{K}_{n'}|}{|\mathbf{K}_{n'-1}|}\right)^{-1/2} \left(\frac{\mathbf{1}_{n'}^T \mathbf{K}_{n'}^{-1} \mathbf{1}_{n'}}{\mathbf{1}_{n'-1}^T \mathbf{K}_{n'-1}^{-1} \mathbf{1}_{n'-1}}\right)^{-1/2} \\
&\quad \times \exp\left(-\frac{1}{2\sigma^2}\left(\mathbf{y}_{(n-1):n}^T \mathbf{M}_{n'} \mathbf{y}_{(n-1):n}\right)\right) d\sigma^2 \\
&\propto \left(\frac{|\mathbf{K}_{n'}|}{|\mathbf{K}_{n'-1}|}\right)^{-1/2} \left(\frac{\mathbf{1}_{n'}^T \mathbf{K}_{n'}^{-1} \mathbf{1}_{n'}}{\mathbf{1}_{n'-1}^T \mathbf{K}_{n'-1}^{-1} \mathbf{1}_{n'-1}}\right)^{-1/2} \left(\mathbf{y}_{(n-1):n}^T \mathbf{M}_{n'} \mathbf{y}_{(n-1):n}\right)^{-1/2}.
\end{aligned} \tag{S9}
$$

Combining Equations (S7) and (S9), we have for $i$ from 1 to $n-1$,

$$
\begin{aligned}
&p\left(y_n \mid \mathbf{y}_{i:(n-1)}, \gamma, \eta\right) = \frac{p\left(\mathbf{y}_{i:n} \mid \gamma, \eta\right)}{p\left(\mathbf{y}_{i:(n-1)} \mid \gamma, \eta\right)} \\
&\propto \begin{cases} \frac{\Gamma(\frac{n'-1}{2})}{\Gamma(\frac{n'-2}{2})} \left(\frac{|\mathbf{K}_{n'}|}{|\mathbf{K}_{n'-1}|}\right)^{-1/2} \left(\frac{\mathbf{1}_{n'}^T \mathbf{K}_{n'}^{-1} \mathbf{1}_{n'}}{\mathbf{1}_{n'-1}^T \mathbf{K}_{n'-1}^{-1} \mathbf{1}_{n'-1}}\right)^{-1/2} \exp\left(-S_{n'}^2\right), & i < n-1 \\ \left(\frac{|\mathbf{K}_{n'}|}{|\mathbf{K}_{n'-1}|}\right)^{-1/2} \left(\frac{\mathbf{1}_{n'}^T \mathbf{K}_{n'}^{-1} \mathbf{1}_{n'}}{\mathbf{1}_{n'-1}^T \mathbf{K}_{n'-1}^{-1} \mathbf{1}_{n'-1}}\right)^{-1/2} \left(\mathbf{y}_{(n-1):n}^T \mathbf{M}_{n'} \mathbf{y}_{(n-1):n}\right)^{-1/2}, & i = n-1 \end{cases}
\end{aligned}
$$

where $S^2_{n'} = \left(\frac{n'-1}{2}\right) \log\left(\mathbf{y}^T_{i:n}\mathbf{M}_{n'}\mathbf{y}_{i:n}\right) - \left(\frac{n'-2}{2}\right) \log\left(\mathbf{y}^T_{i:(n-1)}\mathbf{M}_{n'-1}\mathbf{y}_{i:(n-1)}\right)$ and $\mathbf{M}_{n'} = \mathbf{K}^{-1}_{n'} - \mathbf{K}^{-1}_{n'}\mathbf{1}_{n'}\left(\mathbf{1}^T_{n'}\mathbf{K}^{-1}_{n'}\mathbf{1}_{n'}\right)^{-1}\mathbf{1}^T_{n'}\mathbf{K}^{-1}_{n'}$.

# S5 Kalman Filter for Dynamic Linear Models

Let $Y_k$ be the observations modeled by the DLM for $k = 1, \ldots, n'$, i.e.

$$\begin{aligned} Y_k &= \mathbf{F}_k\boldsymbol{\theta}_k + \epsilon_k \quad \epsilon_k \sim \mathcal{N}\left(0, \sigma_0^2\right) \\ \boldsymbol{\theta}_k &= \mathbf{G}_k\boldsymbol{\theta}_{k-1} + \mathbf{w}_k \quad \mathbf{w}_k \sim \mathcal{MN}\left(0, \mathbf{W}_k\right), \end{aligned} \tag{S10}$$

where $\boldsymbol{\theta}_k$ is a $q$-dimensional latent state process with the initial state $\boldsymbol{\theta}_0 \sim \mathcal{N}(0, \mathbf{B}_0)$. For $k = 1, \ldots, n'$, given $\boldsymbol{\theta}_{k-1} \mid \mathbf{Y}_{1:(k-1)} \sim \mathcal{MN}\left(\mathbf{m}_{k-1}, \mathbf{B}_{k-1}\right)$, we iteratively compute the distribution of $\boldsymbol{\theta}_k$ given $\mathbf{Y}_{1:k}$ by the following three steps (Petris et al., 2009).

First, we compute the one-step-ahead predictive distribution of $\boldsymbol{\theta}_k$ given $\mathbf{Y}_{1:(k-1)}$

$$\boldsymbol{\theta}_k \mid \mathbf{Y}_{1:(k-1)} \sim \mathcal{MN}\left(\mathbf{d}_k, \mathbf{D}_k\right), \tag{S11}$$

with $\mathbf{d}_k = \mathbf{G}_k\mathbf{m}_{k-1}$ and $\mathbf{D}_k = \mathbf{G}_k\mathbf{B}_{k-1}\mathbf{G}^T_k + \mathbf{W}_k$.

Next, we compute the one-step-ahead predictive distribution of $Y_k$ given $\mathbf{Y}_{1:(k-1)}$ below,

$$Y_k \mid \mathbf{Y}_{1:(k-1)} \sim \mathcal{N}\left(f_k, Q_k\right), \tag{S12}$$

with $f_k = \mathbf{F}_k\mathbf{d}_k$, and $Q_k = \mathbf{F}_k\mathbf{D}_k\mathbf{F}^T_k + \sigma_0^2$.

In the last step, we compute the filtering distribution of $\boldsymbol{\theta}_k$ given $\mathbf{Y}_{1:k}$, i.e.,

$$\boldsymbol{\theta}_k \mid \mathbf{Y}_{1:k} \sim \mathcal{MN}\left(\mathbf{m}_k, \mathbf{B}_k\right), \tag{S13}$$

with $\mathbf{m}_k = \mathbf{d}_k + \mathbf{D}_k\mathbf{F}^T_k Q_k^{-1}\left(Y_k - f_k\right)$ and $\mathbf{B}_k = \mathbf{D}_k - \mathbf{D}_k\mathbf{F}^T_k Q_k^{-1}\mathbf{F}_k\mathbf{D}_k$.

# S6 Proof of Lemma 1

*Proof.* Let the observations $\mathbf{Y}_{1:n'} = \left(Y_1, \ldots, Y_{n'}\right)^T$ follow a multivariate normal distribution with covariance matrix $\mathbf{K}_{n'}$, i.e.

$$\mathbf{Y}_{1:n'} \sim \mathcal{MN}(0, \mathbf{K}_{n'}). \tag{S14}$$

The likelihood function of $\mathbf{Y}_{1:n'}$ can be decomposed as follows.

$$\begin{aligned} l(\mathbf{Y}_{1:n'}; \mathbf{K}_{n'}) &= (2\pi)^{-\frac{n'}{2}} |\mathbf{K}_{n'}|^{-\frac{1}{2}} \exp\left(-\frac{1}{2}\mathbf{Y}^T_{1:n'}\mathbf{K}^{-1}_{n'}\mathbf{Y}_{1:n'}\right) \\ &= (2\pi)^{-\frac{n'}{2}} |\mathbf{K}_{n'}|^{-\frac{1}{2}} \exp\left(\frac{1}{2}\mathbf{Y}^T_{1:n'}\mathbf{U}^T_{n'}\mathbf{U}_{n'}\mathbf{Y}_{1:n'}\right) \\ &= (2\pi)^{-\frac{n'}{2}} |\mathbf{K}_{n'}|^{-\frac{1}{2}} \exp\left(\frac{1}{2}\sum_{k=1}^{n'}\left(\mathbf{U}_{n'}\mathbf{Y}_{1:n'}\right)^2_k\right), \end{aligned} \tag{S15}$$

where $(\cdot)_k$ represents the $k$-th element in the vector. The second equation is a result of applying the Cholesky decomposition on the covariance matrix, where $\mathbf{K}_{n'} = \mathbf{L}_{n'}\mathbf{L}_{n'}^T$. Here, $\mathbf{L}_{n'}$ is a lower triangular matrix. Consequently, we have $\mathbf{K}_{n'}^{-1} = \mathbf{U}_{n'}^T\mathbf{U}_{n'}$, with $\mathbf{U}_{n'} = \mathbf{L}_{n'}^{-1}$.

Next, we show that the likelihood function $l(\mathbf{Y}_{1:n'}; \mathbf{K}_{n'})$ in Equation (S15) is a function of the Kalman filter parameters in Section S5. Based on Equation (S12), the predictive distribution of $Y_k$ given $\mathbf{Y}_{1:(k-1)}$ for $k = 2, \dots, n'$ takes the following form.

$$p(Y_k \mid \mathbf{Y}_{1:(k-1)}) \sim \mathcal{N}(f_k, Q_k), \tag{S16}$$

where $f_k$, and $Q_k$ are scalar Kalman filter parameters that can be computed in time complexity $O(1)$ iteratively. We will discuss the details of this computation later in this section. When $k = 1$, based on Equation (S12), we have $p(Y_1) \sim \mathcal{N}(f_1, Q_1)$, where $f_1 = 0$ and $Q_1 = \mathbf{F}_1\mathbf{D}_1\mathbf{F}_1^T + \eta$. Therefore, the likelihood function of $\mathbf{Y}_{1:n'}$ from the Kalman filter follows.

$$\begin{aligned} l(\mathbf{Y}_{1:n'}; \mathbf{K}_{n'}) &= p(Y_1)\prod_{k=2}^{n'} p(Y_k \mid \mathbf{Y}_{1:(k-1)}) \\ &= \prod_{k=1}^{n'} (2\pi)^{-\frac{1}{2}} Q_k^{-\frac{1}{2}} \exp\left(-\frac{1}{2}\frac{(Y_k - f_k)^2}{Q_k}\right) \\ &= (2\pi)^{-\frac{n'}{2}} \prod_{k=1}^{n'} Q_k^{-\frac{1}{2}} \exp\left(-\frac{1}{2}\sum_{k=1}^{n'}\frac{(Y_k - f_k)^2}{Q_k}\right), \end{aligned} \tag{S17}$$

where the first equation is formulated using conditional probability, and the second equation is from Equation (S16). Since Equations (S15) and (S17) are equivalent for any $n' > 0$, terms in Equation (S15) can be replaced by the Kalman Filter parameters in Equation (S17), i.e.

$$|\mathbf{K}_{n'}|^{-\frac{1}{2}} = \prod_{k=1}^{n'} Q_k^{-\frac{1}{2}} \text{ and} \tag{S18}$$

$$(\mathbf{U}_{n'}\mathbf{Y}_{1:n'})_k = \frac{Y_k - f_k}{Q_k^{\frac{1}{2}}} \text{ for any } 1 \le k \le n' \tag{S19}$$

We denote $\mathbf{u}_{n'} = \mathbf{U}_{n'}\mathbf{1}_{n'} = (u_1, \dots, u_{n'})^T$ and $\mathbf{v}_{i,n'} = \mathbf{U}_{n'}\mathbf{y}_{i:n} = (v_{i,1}, \dots, v_{i,n'})^T$. By substituting $\mathbf{Y}_{1:n'}$ in Equation (S19) with $\mathbf{1}_{n'}$ and $\mathbf{y}_{i:n}$, respectively, we have for $k = 1, \dots, n'$,

$$\begin{aligned} u_k = (\mathbf{U}_{n'}\mathbf{1}_{n'})_k &= \frac{1 - f_k^u}{\sqrt{Q_k^u}}, \\ v_{i,k} = (\mathbf{U}_{n'}\mathbf{y}_{i:n})_k &= \frac{y_{i+k-1} - f_{i,k}^v}{\sqrt{Q_{i,k}^v}}, \end{aligned} \tag{S20}$$

where $f_k^u$ and $Q_k^u$ are the Kalman filter parameters when $\mathbf{Y}_{1:n'} = \mathbf{1}_{n'}$ in Equation (S12), and $f_{i,k}^v$ and $Q_{i,k}^v$ are the Kalman filter parameters when $\mathbf{Y}_{1:n'} = \mathbf{y}_{i:n}$.

Next, we discuss in detail the sequential computation process of Kalman filter parameters $f_k^u$, $Q_k^u$, $f_{i,k}^v$ and $Q_{i,k}^v$ for $k = 1, \dots, n'$. Based on Section S5, for the vector $\mathbf{u}_{n'}$, given

the matrics $\mathbf{F}^u_{k-1}$, $\mathbf{G}^u_{k-1}$, $\mathbf{d}^u_{k-1}$ and $\mathbf{D}^u_{k-1}$ at the $(k-1)$-th step and the matrics $\mathbf{F}^u_k$, $\mathbf{G}^u_k$ and $\mathbf{W}^u_k$ at the $k$-th step, we have the updating equations below when $k \geq 2$

$$\begin{aligned}
f^u_k &= \mathbb{E}_{\mathbf{Y}_{1:k}}[Y_k \mid \mathbf{Y}_{1:(k-1)} = \mathbf{1}_{k-1}, \gamma, \eta] \\
&= \mathbf{F}^u_k \mathbf{d}^u_k \\
&= \mathbf{F}^u_k \mathbf{G}^u_k \mathbf{m}^u_{k-1} \\
&= \mathbf{F}^u_k \mathbf{G}^u_k \mathbf{d}^u_{k-1} + \mathbf{F}^u_k \mathbf{G}^u_k \mathbf{D}^u_{k-1} (\mathbf{F}^u_{k-1})^T \frac{1 - f^u_{k-1}}{Q^u_{k-1}} \\
&= g^u_k(f^u_{k-1}, Q^u_{k-1}), \text{ and}
\end{aligned} \tag{S21}$$

$$\begin{aligned}
Q^u_k &= \mathbb{V}_{\mathbf{Y}_{1:k}}[Y_k \mid \mathbf{Y}_{1:(k-1)} = \mathbf{1}_{k-1}, \gamma, \eta] \\
&= \mathbf{F}^u_k \mathbf{D}^u_k (\mathbf{F}^u_k)^T + \sigma_0^2 \\
&= \mathbf{F}^u_k \mathbf{G}^u_k \mathbf{B}^u_{k-1} (\mathbf{F}^u_k \mathbf{G}^u_k)^T + \mathbf{F}^u_k \mathbf{W}^u_k (\mathbf{F}^u_k)^T + \eta \\
&= \beta^u_{1,k} + \beta^u_{2,k} \frac{1}{Q^u_{k-1}} \\
&= h^u_k(Q^u_{k-1}),
\end{aligned} \tag{S22}$$

where $\beta^u_{1,k} = \mathbf{F}^u_k \mathbf{G}^u_k \mathbf{D}^u_{k-1} (\mathbf{F}^u_k \mathbf{G}^u_k)^T + \mathbf{F}^u_k \mathbf{W}^u_k (\mathbf{F}^u_k)^T + \eta$ and $\beta^u_{2,k} = -\left(\mathbf{F}^u_k \mathbf{G}^u_k \mathbf{D}^u_{k-1} (\mathbf{F}^u_{k-1})^T\right)^2$. For $k = 1$, the initialization of $f^u_1$ and $Q^u_1$ from Equation (S12) follows

$$\begin{aligned}
f^u_1 &= 0 \\
Q^u_1 &= \mathbf{F}^u_1 \mathbf{D}^u_1 (\mathbf{F}^u_1)^T + \eta.
\end{aligned} \tag{S23}$$

Similarly, for the vector $\mathbf{v}_{i,n'}$, given the matrics $\mathbf{F}^v_{i,k-1}$, $\mathbf{G}^v_{i,k-1}$, $\mathbf{d}^v_{i,k-1}$ and $\mathbf{D}^v_{i,k-1}$ at the $(k-1)$-th step and the matrics $\mathbf{F}^v_{i,k}$, $\mathbf{G}^v_{i,k}$ and $\mathbf{W}^v_{i,k}$ at the $k$-th step, we have the following updating equations for $k \geq 2$.

$$\begin{aligned}
f^v_{i,k} &= \mathbb{E}_{\mathbf{Y}_{1:k}}[Y_k \mid \mathbf{Y}_{1:(k-1)} = \mathbf{y}_{i:(i+k-2)}, \gamma, \eta] \\
&= \mathbf{F}^v_{i,k} \mathbf{d}^v_{i,k} \\
&= \mathbf{F}^v_{i,k} \mathbf{G}^v_{i,k} \mathbf{m}^v_{i,k-1} \\
&= \mathbf{F}^v_{i,k} \mathbf{G}^v_{i,k} \mathbf{d}^v_{i,k-1} + \mathbf{F}^v_{i,k} \mathbf{G}^v_{i,k} \mathbf{D}^v_{i,k-1} (\mathbf{F}^v_{i,k-1})^T \frac{y_{i+k-2} - f^v_{i,k-1}}{Q^v_{i,k-1}} \\
&= g^v_{i,k}(f^v_{i,k-1}, Q^v_{i,k-1}), \text{ and}
\end{aligned} \tag{S24}$$

$$\begin{aligned}
Q^v_{i,k} &= \mathbb{V}_{\mathbf{Y}_{1:k}}[Y_k \mid \mathbf{Y}_{1:(k-1)} = \mathbf{y}_{i:(i+k-2)}, \gamma, \eta] \\
&= \mathbf{F}^v_{i,k} \mathbf{D}^v_{i,k} (\mathbf{F}^v_{i,k})^T + \sigma_0^2 \\
&= \mathbf{F}^v_{i,k} \mathbf{G}^v_{i,k} (\mathbf{F}^v_{i,k} \mathbf{G}^v_{i,k} \mathbf{B}^v_{i,k-1})^T + \mathbf{F}^v_{i,k} \mathbf{W}^v_{i,k} (\mathbf{F}^v_{i,k})^T + \sigma_0^2 \\
&= \beta^v_{1,i,k} + \beta^v_{2,i,k} \frac{1}{Q^v_{i,k-1}} \\
&= h^v_{i,k}(Q^v_{i,k-1}),
\end{aligned} \tag{S25}$$

where $\beta^v_{1,i,k} = \mathbf{F}^v_{i,k}\mathbf{G}^v_{i,k}\mathbf{D}^v_{i,k-1}(\mathbf{F}^v_{i,k}\mathbf{G}^v_{i,k})^T + \mathbf{F}^v_{i,k}\mathbf{W}^v_{i,k}(\mathbf{F}^v_{i,k})^T + \sigma_0^2$ and $\beta^v_{2,i,k} = -(\mathbf{F}^v_{i,k}\mathbf{G}^v_{i,k}\mathbf{D}^v_{i,k-1}(\mathbf{F}^v_{i,k-1})^T)^2$. For $k=1$, the initialization of $f^u_1$ and $Q^u_1$ from Equation (S12) follows

$$\begin{aligned} f^v_{i,1} &= 0, \\ Q^v_{i,1} &= \mathbf{F}^v_{i,1}\mathbf{D}^v_{i,1}(\mathbf{F}^v_{i,1})^T + \eta. \end{aligned} \tag{S26}$$

□

# S7 Proof of Theorem 1

*Proof.* The fast computation of the predictive distribution $p\left(y_n \mid \mathbf{y}_{i:(n-1)}, \gamma, \eta\right)$ can be achieved by sequential Kalman filter. By applying the Cholesky decomposition on the covariance matrix $\mathbf{K}_{n'}$, we have $\mathbf{K}_{n'} = \mathbf{L}_{n'}\mathbf{L}^T_{n'}$, where $\mathbf{L}_{n'}$ is a lower triangular matrix, and $\mathbf{K}^{-1}_{n'} = \mathbf{U}^T_{n'}\mathbf{U}_{n'}$ with $\mathbf{U}_{n'} = \mathbf{L}^{-1}_{n'}$. Then, by denoting $\mathbf{u}_{n'} = \mathbf{U}_{n'}\mathbf{1}_{n'} = (u_1, \ldots, u_{n'})^T$ and $\mathbf{v}_{i,n'} = \mathbf{U}_{n'}\mathbf{y}_{i:n} = (v_{i,1}, \ldots, v_{i,n'})^T$, we have the following equations.

$$\begin{aligned} \mathbf{1}^T_{n'}\mathbf{K}^{-1}_{n'}\mathbf{1}_{n'} &= \mathbf{1}^T_{n'}\mathbf{U}^T_{n'}\mathbf{U}_{n'}\mathbf{1}_{n'} = \mathbf{u}^T_{n'}\mathbf{u}_{n'}, \\ \mathbf{y}^T_{i:n}\mathbf{K}^{-1}_{n'}\mathbf{y}_{i:n} &= \mathbf{y}^T_{i:n}\mathbf{U}^T_{n'}\mathbf{U}_{n'}\mathbf{y}_{i:n} = \mathbf{v}^T_{i,n'}\mathbf{v}_{i,n'}, \\ \mathbf{y}^T_{i:n}\mathbf{K}^{-1}_{n'}\mathbf{1}_{n'} &= \mathbf{y}^T_{i:n}\mathbf{U}^T_{n'}\mathbf{U}_{n'}\mathbf{1}_{n'} = \mathbf{v}^T_{i,n'}\mathbf{u}_{n'}, \\ \frac{|\mathbf{K}_{n'}|}{|\mathbf{K}_{n'-1}|} &= \frac{\Pi^{n'}_{k=1}Q^u_k}{\Pi^{n'-1}_{k=1}Q^u_k} = Q^u_{n'}, \end{aligned} \tag{S27}$$

where the last equation is derived based on Equation (S18).

Given the Equation (S27), the predictive distribution $p\left(y_n \mid \mathbf{y}_{i:(n-1)}, \gamma, \eta\right)$ in Equation (7) can be represented using the two vectors $\mathbf{u}_{n'}$ and $\mathbf{v}_{i,n'}$. For $i < n-1$, we have

$$\begin{aligned}
&p\left(y_n \mid \mathbf{y}_{i:(n-1)}, \gamma, \eta\right) \\
&\propto \frac{\Gamma\left(\frac{n'-1}{2}\right)}{\Gamma\left(\frac{n'-2}{2}\right)} \left(\frac{|\mathbf{K}_{n'}|}{|\mathbf{K}_{n'-1}|}\right)^{-1/2} \left(\frac{\left|\mathbf{1}^T_{n'}\mathbf{K}^{-1}_{n'}\mathbf{1}_{n'}\right|}{\left|\mathbf{1}^T_{n'-1}\mathbf{K}^{-1}_{n'-1}\mathbf{1}_{n'-1}\right|}\right)^{-1/2} \frac{\left(\mathbf{y}^T_{i:n}\mathbf{M}_{n'}\mathbf{y}_{i:n}\right)^{-\frac{n'-1}{2}}}{\left(\mathbf{y}^T_{i:(n-1)}\mathbf{M}_{n'-1}\mathbf{y}_{i:(n-1)}\right)^{\frac{-n'-2}{2}}} \\
&\propto \frac{\Gamma\left(\frac{n'-1}{2}\right)}{\Gamma\left(\frac{n'-2}{2}\right)} \left(\frac{|\mathbf{K}_{n'}|}{|\mathbf{K}_{n'-1}|}\right)^{-1/2} \left(\frac{\left|\mathbf{1}^T_{n'}\mathbf{K}^{-1}_{n'}\mathbf{1}_{n'}\right|}{\left|\mathbf{1}^T_{n'-1}\mathbf{K}^{-1}_{n'-1}\mathbf{1}_{n'-1}\right|}\right)^{-1/2} \\
&\quad\times \frac{\left(\mathbf{y}^T_{i:n}\mathbf{K}^{-1}_{n'}\mathbf{y}_{i:n} - \mathbf{y}^T_{i:n}\mathbf{K}^{-1}_{n'}\mathbf{1}_{n'}\left(\mathbf{1}^T_{n'}\mathbf{K}^{-1}_{n'}\mathbf{1}_{n'}\right)^{-1}\mathbf{1}^T_{n'}\mathbf{K}^{-1}_{n'}\mathbf{y}_{i:n}\right)^{-\frac{n'-1}{2}}}{\left(\mathbf{y}^T_{i:(n-1)}\mathbf{K}^{-1}_{n'-1}\mathbf{y}_{i:(n-1)} - \mathbf{y}^T_{i:(n-1)}\mathbf{K}^{-1}_{n'-1}\mathbf{1}_{n'-1}\left(\mathbf{1}^T_{n'-1}\mathbf{K}^{-1}_{n'-1}\mathbf{1}_{n'-1}\right)^{-1}\mathbf{1}^T_{n'-1}\mathbf{K}^{-1}_{n'-1}\mathbf{y}_{i:(n-1)}\right)^{-\frac{n'-2}{2}}} \\
&\propto \frac{\Gamma\left(\frac{n'-1}{2}\right)}{\Gamma\left(\frac{n'-2}{2}\right)} (Q^u_{n'})^{-1/2} \left(\frac{\mathbf{u}^T_{n'}\mathbf{u}_{n'}}{\mathbf{u}^T_{n'-1}\mathbf{u}_{n'-1}}\right)^{-1/2} \\
&\quad\times \frac{\left(\mathbf{v}^T_{i,n'}\mathbf{v}_{i,n'} - \mathbf{v}^T_{i,n'}\mathbf{u}_{n'}\left(\mathbf{u}^T_{n'}\mathbf{u}_{n'}\right)^{-1}\mathbf{u}^T_{n'}\mathbf{v}_{i,n'}\right)^{-\frac{n'-1}{2}}}{\left(\mathbf{v}^T_{i,n'-1}\mathbf{v}_{i,n'-1} - \mathbf{v}^T_{i,n'-1}\mathbf{u}_{n'-1}\left(\mathbf{u}^T_{n'-1}\mathbf{u}_{n'-1}\right)^{-1}\mathbf{u}^T_{n'-1}\mathbf{v}_{i,n'-1}\right)^{-\frac{n'-2}{2}}} \\
&\propto \frac{\Gamma\left(\frac{n'-1}{2}\right)}{\Gamma\left(\frac{n'-2}{2}\right)} (Q^u_{n'})^{-1/2} \left(\frac{\mathbf{u}^T_{n'}\mathbf{u}_{n'}}{\mathbf{u}^T_{n'-1}\mathbf{u}_{n'-1}}\right)^{-1/2} \exp\left(-S^2_{n'}\right),
\end{aligned}$$

Table S1: Comparisons of time complexity between SKF and other online changepoint detection methods for detecting the most recent changepoint when there are $n$ observations.

| Method | Computational complexity | Temporal correlation | Allow detecting variance change |
|---|---|---|---|
| Cumulative sum chart (Page, 1954) | $\mathcal{O}(1)$ | No | No |
| Bayesian online changepoint detection (Fearnhead and Liu, 2007) (Adams and MacKay, 2007) | $\mathcal{O}(n)$ | No | Yes |
| Bayesian analysis with dependence across regimes (Fearnhead and Liu, 2011) | $\mathcal{O}(n)$ | Dependence across segments | No |
| Detecting abrupt changes (Romano et al., 2022) | $\mathcal{O}(n)$ | Dependence from autocorrelated noise | No |
| Gaussian process changepoint detection (Saatçi et al., 2010) | $\mathcal{O}(n^3)$ | Dependence within segments | Yes |
| SKF | $\mathcal{O}(n')$ | Dependence within segments | Yes |

where $S_{n'}^2 = \left(\frac{n'-1}{2}\right) \log\left(\mathbf{y}_{i:n}^T \mathbf{M}_{n'} \mathbf{y}_{i:n}\right) - \left(\frac{n'-2}{2}\right) \log\left(\mathbf{y}_{i:(n-1)}^T \mathbf{M}_{n'-1} \mathbf{y}_{i:(n-1)}\right)$, and $\mathbf{y}_{i:n}^T \mathbf{M}_{n'} \mathbf{y}_{i:n} = \mathbf{v}_{i,n'}^T \mathbf{v}_{i,n'} - \left(\mathbf{u}_{n'}^T \mathbf{u}_{n'}\right)^{-1} \left(\mathbf{v}_{i,n'}^T \mathbf{u}_{n'}\right)^2$. The third proportion is derived based on Equation (S27). For $i = n-1$, similarly we have

$$
\begin{aligned}
& p(y_n \mid \mathbf{y}_{i:(n-1)}, \gamma, \eta) \\
& \propto \left(\frac{|\mathbf{K}_{n'}|}{|\mathbf{K}_{n'-1}|}\right)^{-1/2} \left(\frac{\left|\mathbf{1}_{n'}^T \mathbf{K}_{n'}^{-1} \mathbf{1}_{n'}\right|}{\left|\mathbf{1}_{n'-1}^T \mathbf{K}_{n'-1}^{-1} \mathbf{1}_{n'-1}\right|}\right)^{-1/2} \left(\mathbf{y}_{(n-1):n}^T \mathbf{M}_{n'} \mathbf{y}_{(n-1):n}\right)^{-\frac{1}{2}} \\
& \propto \left(Q_{n'}^u\right)^{-\frac{1}{2}} \left(\frac{\mathbf{u}_{n'}^T \mathbf{u}_{n'}}{\mathbf{u}_{n'-1}^T \mathbf{u}_{n'-1}}\right)^{-1/2} \left(\mathbf{y}_{i:n}^T \mathbf{M}_{n'} \mathbf{y}_{i:n}\right)^{-1/2}.
\end{aligned}
$$

The main advantage of expressing the predictive distribution $p\left(y_n \mid \mathbf{y}_{i:(n-1)}, \gamma, \eta\right)$ in terms of vectors $\mathbf{u}_{n'}$ and $\mathbf{v}_{i,n'}$ is the reduction of computational complexity. Based on Equation (S20), vectors $\mathbf{u}_{n'}$ and $\mathbf{v}_{i,n'}$ can be sequentially updated from $\mathbf{u}_{n'-1}$ and $\mathbf{v}_{i,n'-1}$ with only $\mathcal{O}(1)$ operations. Consequently, when written as functions of $\mathbf{u}_{n'}$ and $\mathbf{v}_{i,n'}$, the predictive distribution $p\left(y_n \mid \mathbf{y}_{i:(n-1)}, \gamma, \eta\right)$ can also be sequentially computed in $\mathcal{O}(1)$ operations.

□

# S8 Comparison and Connection with Other Models

We compare various online changepoint detection methods in Table S1. For instance, the cumulative sum (CUSUM) chart (Page, 1954; Kurt et al., 2020) and BOCPD methods do not consider temporal correlation in the data. To address this issue, Fearnhead and Liu (2011) introduces a piecewise polynomial regression model that considers temporal correlations between segments, yet this method doesn't model the temporal correlation

within each segment, an aspect our approach effectively handles. Additionally, Romano et al. (2022) specifically targets detecting mean shifts in time series with autocorrelated noise. However, our proposed approach can detect both mean and variance shifts, making it a more flexible solution for changepoint detection.

The GPCPD method (Saatçi et al., 2010) models correlation between observations at each time point, whereas it has a large computational cost. In comparison, the computational complexity of SKF scales linearly to the number of observations between the most recent changepoints and the previous changepoint in the SKF algorithm. Furthermore, the mean and variance are efficiently integrated out in SKF based on the most recent observations, which makes it particularly suitable for online changepoint detection.

Other techniques to reduce computational complexity include rank 1 update (Schölkopf and Smola, 2018), which has higher computational complexity than SKF. Another approach to reduce the computational complexity is to factorizing the semi-separable covariance matrix in a backward recursive algorithm (Gu et al., 2013). The SKF has two advantages over this approach. First, we integrate out mean and variance parameters in SKF, which is crucial for computing the predictive distribution based on the latest information for changepoint detection. Secondly, the SKF algorithm is applicable to all dynamical linear models that go beyond the Gaussian process with a Matérn kernel.

# S9 The CUSUM Algorithm

The cumulative sum (CUSUM) control chart is an online changepoint detection algorithm proposed by Page (1954). Denote $y_1, \ldots, y_n$ as observations from time $t_1$ to $t_n$. We define $y_j^* = \frac{y_j - \bar{y}_{1:j}}{\hat{\sigma}_{1:j}}$ as standardized observations for $j = 1, \ldots, n$, where the $\bar{y}_{1:j}$ and $\hat{\sigma}_{1:j}$ are the sample mean and standard deviation for all the observations until time $t_j$, respectively. A changepoint is detected at time $t_n$ if either of the two CUSUM statistics conditions are met, i.e.,

$$S_n^+ > h \text{ or } S_n^- < -h, \tag{S28}$$

where

$$\begin{aligned} S_n^+ &= \max(0, S_{n-1}^+ + y_n^* - K_n), \\ S_n^- &= -\max(0, S_{n-1}^- - y_n^* + K_n), \end{aligned} \tag{S29}$$

are the upper and lower CUSUM statistics at time $t_n$, respectively. The parameters $K_n$ and $h$ control the sensitivity of the CUSUM method to detect the changepoints. Specifically, the parameter $K_n$ is the deviation between the normalized observations $y_n^*$ and the standardized mean zero that we wish to detect. For example, $K_n = 0.5$ indicates that the mean shift we aim to detect for the normalized observations $y_n^*$ is at least 0.5. Similarly, the parameter $h$ controls the distance between the CUSUM statistics and the baseline zero we want to detect. In both simulations and real data analysis, we tune parameters $K_n$ and $h$ to control type-I errors during training. Once set, these parameters remain constant when identifying change points on testing samples.

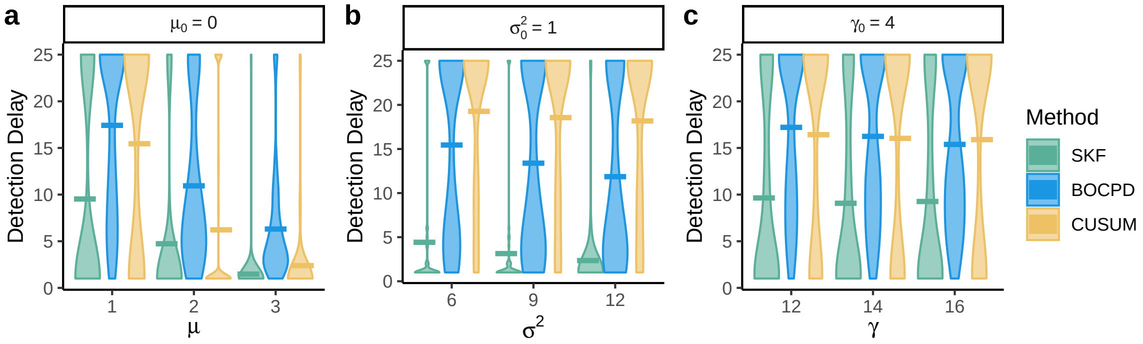


Figure S3: Violin plots comparing average detection delay for SKF, BOCPD, and CUSUM methods for 100 simulations. The data are simulated with the Matérn correlation and the roughness parameter being 2.5, while we use **misspecified** Exponential correlation in the SKF method to detect changepoints. A method with a low average detection delay is better. $\mu_0$, $\sigma_0^2$ and $\gamma_0$ represent pre-change parameter values, while $\mu$, $\sigma^2$ and $\gamma$ on the x-axis stand for post-change parameter values.

# S10 Simulation Studies with Misspecified Configurations

To test the robustness of the SKF method, we perform simulated studies under misspecified conditions, using data from a GP model having a Matérn covariance function with roughness parameter being 2.5 while employing an Exponential correlation in the SKF algorithm for changepoint detection. For comparison, we also implemented the BOCPD and CUSUM methods, using the configurations from Section 3.1. This involves considering three types of changes, including changes in mean, variance, and correlation. For each configuration, 100 simulation experiments are conducted. In each of these, 100 observations are generated, with the initial 50 serving as training samples. The true changepoint is set at time 75, and we record the average detection delay for all methods.

Figure S3 shows the average detection delay for the misspecified SKF method, the BOCPD method, and the CUSUM method. Notably, even when misspecified, the SKF method consistently outperforms the other methods with a lower average detection delay. The better performance of the SKF method, even with a misspecified correlation function, can likely be attributed to its ability to recognize and capture temporal correlations within the data. This ability enables the SKF method to avoid detecting false changepoints from large fluctuations caused by these temporal correlations, thereby reducing false detections. In contrast, methods such as BOCPD and CUSUM are not able to account for these temporal correlations, potentially leading to a higher rate of false positives. Given that we maintained a consistent type-I error rate across all methods during training, BOCPD and CUSUM required larger hazard parameters due to their increased sensitivity to false positives, resulting in higher average detection delays compared to SKF.

# S11 Definition of the Covering Metric

Define the ordered set of latent true changepoints as $\boldsymbol{\tau} = \{\tau_1, \ldots, \tau_{m_1}\}$, where $\tau_i$ takes values in time indices $1, \ldots, n$ and $\tau_i < \tau_j$ for $i < j$. This ordered set $\boldsymbol{\tau}$ induces a partition $\mathcal{G}$, separating the interval $[t_1, t_n]$ into $m_1 + 1$ disjoint sets $\boldsymbol{A} = \{\mathcal{A}_1, \ldots, \mathcal{A}_{m_1+1}\}$. The ordered set of detected changepoints is denoted as $\hat{\boldsymbol{\tau}} = \{\hat{\tau}_1, \ldots, \hat{\tau}_{m_2}\}$, where $m_2$ may not be the same as $m_1$. The partition induces by $\hat{\boldsymbol{\tau}}$ is denoted as $\mathcal{G}'$, with the corresponding disjoint set represented as $\boldsymbol{A}' = \left\{\mathcal{A}'_1, \ldots, \mathcal{A}'_{m_2+1}\right\}$. The *covering metric* between two partitions is defined as:

$$C(\mathcal{G}, \mathcal{G}') = \frac{1}{n} \sum_{i=1}^{m_1+1} |\mathcal{A}_i| \max_{1 \leq j \leq m_2+1} J(\mathcal{A}_i, \mathcal{A}'_j), \tag{S30}$$

where $|\mathcal{A}_i|$ represents the number of observations in $\mathcal{A}_i$, and $J(\mathcal{A}_i, \mathcal{A}'_j) = \frac{\left|\mathcal{A}_i \cap \mathcal{A}'_j\right|}{\left|\mathcal{A}_i \cup \mathcal{A}'_j\right|}$ is the Jaccard index.

# S12 An Integrated Algorithm to Detect the COVID-19 Infection

**Algorithm S1** An integrated algorithm to detect COVID-19 infection

**Require:** Logit transformation of classification probabilities $\{y_t\}_{t=1}^n$ from a classification model, such as XGBoost.

**Ensure:** A set of detected changepoints $\hat{\boldsymbol{\tau}}$.

1: Estimate the range parameter and nugget parameter $(\hat{\gamma}, \hat{\eta})$ by maximizing the marginal likelihood across all the patients using $n_0$ training time points, after integrating out the distinct mean and variance parameters for each patient.

2: Apply SKF in Algorithm 1 using $n_0$ training time points to control the type-I error to be 0.4%, the baseline COVID-19 positive proportion.

3: **for** $j$ in $(n_0 + 1) : n$ of each patient **do**

4: Run Algorithm 1 on the observations $\mathbf{y}_{(n_0+1):j}$ to obtain $\hat{C}_j$, the most recently detected changepoint before or at time $t_j$.

5: When the detected changepoint $\hat{C}_j$ is within seven days before the current time $t_j$, i.e. $t_j - \hat{C}_j \leq 7$, we test the following hypothesis to identify the increasing subsequence:

$$H_0 : \mu_1 = \mu_2 \text{ vs } H_a : \mu_1 < \mu_2,$$

where $\mu_1$ and $\mu_2$ are the mean of the subsequences $\mathbf{y}_{(n_0+1):(\hat{C}_j-1)}$ and $\mathbf{y}_{\hat{C}_j:j}$. When the test statistics in Equation (S34) of supplementary material fall into a rejection region, we add the value of $\hat{C}_j$ to the changepoint set $\hat{\boldsymbol{\tau}}$ and mark the 7-day period following the changepoint $\hat{C}_j$, i.e. $t \in [\hat{C}_j, \hat{C}_j + 7]$, as COVID-19 positive for this patient.

6: **end for**

An integrated procedure to detect the changepoint from the COVID-19 infection is summarized in Algorithm S1. We first apply a data-driven classification model to patients' clinical data, here chosen as the XGBoost method (Chen and Guestrin, 2016), which was

previously found to be accurate in detecting COVID-19 among dialysis patients (Monaghan et al., 2021; Duan et al., 2023) compared to a few other statistical learning algorithms. In principle, our changepoint detection method can be applied along with any statistical learning method that gives classification probabilities. We also implemented other statistical learning methods, such as logistic regression and random forests (Breiman, 2001), for baseline comparisons. All methods were trained on longitudinal data from 20% of randomly selected patients, encompassing four million observations. For all approaches, we apply the logit transformation to the probability sequences for mapping the outcomes to the real line. We found that the estimated probabilities of infection are rarely 0 or 1. To prevent numerical errors in the logit transformation, one may replace 0 and 1 with the smallest and largest estimated probabilities within (0,1), respectively.

Second, we apply SKF to detect the change in the daily prediction probabilities of COVID-19 infection from a classification approach, chosen to be XGBoost herein. For demonstration purposes, we compared different approaches for patients with $n > 150$ samples, where the first $n_0 = 100$ samples, labeled as COVID-19 negative, are used as training data to estimate the parameters in changepoint detection approaches, and the remaining samples are used as testing data to evaluate the detection performance. We use an exponential covariance in (4) with the shared range and nugget parameters across patients estimated by maximizing the likelihood of all patients in the training data set, which can improve estimation stability (Gu and Berger, 2016). The mean and variance parameters for different patients and segments are allowed to be distinct, and these parameters are integrated out when computing marginal likelihood and predictive distributions. The distinct mean and variance parameters are flexible for modeling longitudinal observations from a large number of patients.

For both BOCPD and SKF, we utilized the county-level daily Probability of Contracting (PoC) COVID-19 (Li and Gu, 2021) for specifying the hazard function, which is used to control the type I error, described in Step 2 in Algorithm S1. The time-dependent PoC quantifies the average daily COVID-19 transmission probability at the county level among susceptible individuals base on the daily infection and death counts. We found that specifying the hazard function proportional to PoC improves the detection accuracy with a constant hazard function.

Furthermore, we developed an additional screening step to detect the onset of an increasing subsequence in infection probabilities through a hypothesis test (Step 5 in Algorithm S1), as typically the increase of the probability sequences of infection should be detected. Once the detected changepoint passes this screening step, we mark the seven-day period after the detected changepoint as COVID-19 positive (Hakki et al., 2022). The integrated approach is generally applicable to detect changes from longitudinal data.

Next, we show the derivation of the test statistic in Step 5 of Algorithm S1. Denote the test dataset from time $t_{n_0+1}$ to $t_j$ as $\mathbf{y}_{n_0+1:j}$, where $t_{n_0+1}$ is the start time of the testing samples and $j \geq n_0 + 1$. At the time $t_j$, if the estimated most recent changepoint $\hat{C}_j$ satisfies that $\hat{C}_j > n_0 + 1$ and $|t_j - \hat{C}_j| \leq 7$, we test the following hypothesis to identify if $\hat{C}_j$ is a valid changepoint, meaning that the subsequences around $\hat{C}_j$, i.e. $\mathbf{y}_{n_0+1:\hat{C}_j-1}$ and $\mathbf{y}_{\hat{C}_j:j}$, have an increasing trend. We assume that $\mathbf{y}_{n_0+1:\hat{C}_j-1} \sim \mathcal{MN}(\mu_1\mathbf{1}, \sigma^2\mathbf{K}_{n'_1})$ and $\mathbf{y}_{\hat{C}_j:j} \sim \mathcal{MN}(\mu_2\mathbf{1}, \sigma^2\mathbf{K}_{n'_2})$, where $n'_1 = \hat{C}_j - n_0 - 1$, $n'_2 = j - \hat{C}_j + 1$, and test the following

hypothesis.

$$H_0 : \mu_1 = \mu_2 \text{ vs } H_a : \mu_1 < \mu_2.$$

The generalized least square estimators for the mean parameters are as follows.

$$\begin{aligned}\hat{\mu}_1 &= \left(\mathbf{1}^T \hat{\mathbf{K}}_{n_1'}^{-1} \mathbf{1}\right)^{-1} \mathbf{1}^T \hat{\mathbf{K}}_{n_1'}^{-1} \mathbf{y}_{(n_0+1):(\hat{C}_j-1)}, \\ \hat{\mu}_2 &= \left(\mathbf{1}^T \hat{\mathbf{K}}_{n_2'}^{-1} \mathbf{1}\right)^{-1} \mathbf{1}^T \hat{\mathbf{K}}_{n_2'}^{-1} \mathbf{y}_{\hat{C}_j:j},\end{aligned}$$

where the covariance matrices $\hat{\mathbf{K}}_{n_1'}$ and $\hat{\mathbf{K}}_{n_2'}$ are determined using range and nugget parameters $\hat{\gamma}$ and $\hat{\eta}$ estimated from the training samples $\mathbf{y}_{1:n_0}$.

Under the null hypothesis, we have

$$\hat{\mu}_2 - \hat{\mu}_1 \sim \mathcal{MN}(\mu^*, (\sigma^*)^2), \tag{S31}$$

where

$$\begin{aligned}\mu^* &= \mathbb{E}[\hat{\mu}_2] - \mathbb{E}[\hat{\mu}_1] = \mu_2 - \mu_1 = 0, \\ (\sigma^*)^2 &= \mathbb{V}[\hat{\mu}_1] + \mathbb{V}[\hat{\mu}_2] \\ &= \sigma^2 \left( \left(\mathbf{1}^T \hat{\mathbf{K}}_{n_1'}^{-1} \mathbf{1}\right)^{-1} + \left(\mathbf{1}^T \hat{\mathbf{K}}_{n_2'}^{-1} \mathbf{1}\right)^{-1} \right). \end{aligned} \tag{S32}$$

Therefore the test statistic has the following form when we assume the variance $\sigma^2$ and the covariance matrix $\mathbf{K}_1$ and $\mathbf{K}_2$ are known.

$$z = \frac{\hat{\mu}_2 - \hat{\mu}_1 - \mu^*}{\sqrt{(\sigma^*)^2}} = \frac{\hat{\mu}_2 - \hat{\mu}_1}{\sqrt{\sigma^2 \left( \left(\mathbf{1}^T \hat{\mathbf{K}}_{n_1'}^{-1} \mathbf{1}\right)^{-1} + \left(\mathbf{1}^T \hat{\mathbf{K}}_{n_2'}^{-1} \mathbf{1}\right)^{-1} \right)}}, \tag{S33}$$

Under the null hypothesis, $z \sim \mathcal{N}(0, 1)$. In the real data analysis, we estimate the parameters, including the variance $\sigma^2$, the range parameter $\gamma$, and nugget parameter $\eta$ in the covariance matrix $\hat{\mathbf{K}}_{n_1'}$ and $\hat{\mathbf{K}}_{n_2'}$, from the training data. Therefore, by plugging the parameters estimated from the training data into the test statistic $z$ in Equation (S33), we get the following test statistic.

$$z = \frac{\hat{\mu}_2 - \hat{\mu}_1}{\sqrt{\hat{\sigma}^2 \left( \left(\mathbf{1}^T \hat{\mathbf{K}}_{n_1'}^{-1} \mathbf{1}\right)^{-1} + \left(\mathbf{1}^T \hat{\mathbf{K}}_{n_2'}^{-1} \mathbf{1}\right)^{-1} \right)}}, \tag{S34}$$

where

$$\begin{aligned}\hat{\sigma}^2 &= \frac{1}{n-1} \left(\mathbf{y}_{1:n_0} - \mathbf{1}\hat{\mu}_0\right)^T \hat{\mathbf{K}}_{n_0}^{-1} \left(\mathbf{y}_{1:n_0} - \mathbf{1}\hat{\mu}_0\right), \\ \hat{\mu}_0 &= \left(\mathbf{1}^T \hat{\mathbf{K}}_{n_0}^{-1} \mathbf{1}\right)^{-1} \mathbf{1}^T \hat{\mathbf{K}}_{n_0}^{-1} \mathbf{y}_{1:n_0}\end{aligned}$$

The range and nugget parameters $(\hat{\gamma}, \hat{\eta})$ are plugged into covariance matrices to obtain $\hat{\mathbf{K}}_{n_1'}$ and $\hat{\mathbf{K}}_{n_2'}$. As the sample size in the training period is large, we approximate the threshold of the test statistic by normal approximation. We assume normal approximation for the threshold of the test statistic $z$ when comparing the means of two long subsequences, $\mathbf{y}_{(n_0+1):(\hat{C}_j-1)}$ and $\mathbf{y}_{\hat{C}_j:j}$. The robustness of our approach is maintained by the hazard parameter in the SKF method, ensuring Type I error control irrespective of the threshold choice.

Table S2: Comparisons of the statistical learning methods and online changepoint detection methods, including CUSUM, BOCPD, and SKF on COVID-19 patient predictions with the baseline positive rate of 0.4%. The COVID-19 positive period starts on day -4.

| | Precision | Recall | F1-score | Detection Delay |
|---|---|---|---|---|
| Logistic Regression | 0.055 | 0.133 | 0.077 | 1.538 |
| Random Forest | 0.087 | 0.125 | 0.087 | 2.086 |
| XGBoost | 0.082 | 0.179 | 0.113 | 1.799 |
| CUSUM | 0.032 | 0.020 | 0.025 | 3.142 |
| BOCPD | 0.200 | 0.154 | 0.174 | 4.856 |
| SKF | 0.268 | 0.145 | 0.188 | 3.886 |
| SKF with screening | 0.231 | 0.164 | 0.192 | 2.395 |

# S13 Sensitivity Analysis

We show the sensitivity analysis on the definition of the COVID-19 positive period. In the COVID-19 analysis described in Section 4, we defined the positive period from day -2 to day 7, with day 0 being the date the patient received a COVID-19 PCR test. This choice was driven by the average incubation period of COVID-19 infection, which is approximately 3 days (Jansen et al., 2021; Song et al., 2022) before symptoms onset. However, this incubation period may vary among patients.

In this sensitivity analysis, we expanded the definition of the COVID-19 positive period to be from day -4 to day 7. The results of this analysis are shown in Table S2. Notably, the comparative performance of the SKF and BOCPD methods remains consistent with our findings in Section 4. Specifically, the SKF and BOCPD methods continue to outperform all the statistical learning methods and the CUSUM method in terms of the F1-score. It could be attributed to their ability to utilize retrospective information through the recursive computation of the predictive distribution at each time step, as described in Equation (7). Furthermore, consistent with the conclusion we draw from Table 1, the SKF method displayed a lower detection delay and a higher F1-score than the BOCPD method, which can be attributed to SKF's ability to capture the temporal correlations within time segments. These findings suggest that the performance of the changepoint methods is not sensitive to the specific choice of the start date for the COVID-19-positive period.

# S14 More Numerical Comparisons on Real-world Datasets

In this section, we apply the SKF method and other classic online change point detection methods on a set of benchmark datasets in van den Burg and Williams (2020), which includes 37 time series from various domains with ground truth change points annotated by five human annotators. We select eight datasets with a relatively large number of observations and relatively strong temporal correlations to compare our SKF method with other changepoint detection methods. The training data is created from the initial 50 observations of each series, ensuring no changepoints are present. The distribution parameters for SKF and BOCPD are estimated by maximizing the likelihood function on the training data. The hazard parameters for all three changepoint methods are selected so that there

Table S3: Covering metric comparison for SKF, BOCPD and CUSUM. The highest values in each row are in bold type.

| Dataset | SKF | BOCPD | CUSUM |
|---|---|---|---|
| brent_spot | **0.602** | 0.383 | 0.535 |
| businv | **0.814** | 0.471 | 0.510 |
| construction | **0.719** | 0.398 | 0.506 |
| iceland_tourism | 0.624 | **0.685** | 0.617 |
| jfk_passengers | 0.843 | **0.847** | 0.687 |
| lga_passengers | **0.591** | 0.456 | 0.496 |
| quality_control_4 | **0.561** | 0.552 | 0.442 |
| seatbelts | 0.585 | **0.635** | 0.573 |

is no changepoint detected on the training data. All estimated parameters are then applied to the test data to detect changepoints. As each time series may contain multiple changepoints, we utilize the covering metric defined in Section (3.2) to evaluate the performance of the CPD methods. Although all the real datasets are already collected at the time of testing, we apply the SKF as though data points are observed sequentially.

Table S3 shows the covering metric of the SKF and other CPD methods on the eight real datasets. The SKF method has the best covering metric in five out of eight datasets, indicating its capability of detecting changepoints on temporally correlated data. We highlight the functionality of the SKF method by discussing the `businv` dataset. This dataset, sourced from the U.S. Census Bureau, contains the monthly total business inventories in U.S. dollars from 1992 to 2019. It tracks the combined value of goods held by manufacturers, wholesalers, and retailers each month, serving as an important indicator of the health of the supply chain. Five human annotators in van den Burg and Williams (2020) identified seven distinct actual change points within this data, which fall into two categories: (1) **dot-com crush**: changepoints in 2002 marks the end of the dot-com bubble; (2) **financial crisis**: the remaining change points in 2008 indicate the decline in total business inventories caused by the financial crisis.

We fitted a GP model on data from 1992 to 1996 to estimate the variance parameter $\sigma^2$, range parameter $\gamma$, and nugget parameter $\eta$. With these estimations, we employed the SKF method in the following years to detect the changepoints. The estimated changepoints, shown as red crossings in panel a of Figure S4, match well with the actual changepoints related to the two major events, the dot-com crash, and the financial crisis. Further, panel b of this figure shows the posterior distribution of the most recent changepoints, with the red dashed line indicating the location of the changepoints at each time. Regarding the results in Table S3, the SKF on the business inventory dataset outperforms the BOCPD and CUSUM methods for the covering metric, which can be attributed to the model of temporal correlation in the SKF method which was not considered in BOCPD and CUSUM models.

# References

Adams, R. P. and D. J. MacKay (2007). Bayesian online changepoint detection. *arXiv preprint arXiv:0710.3742*.

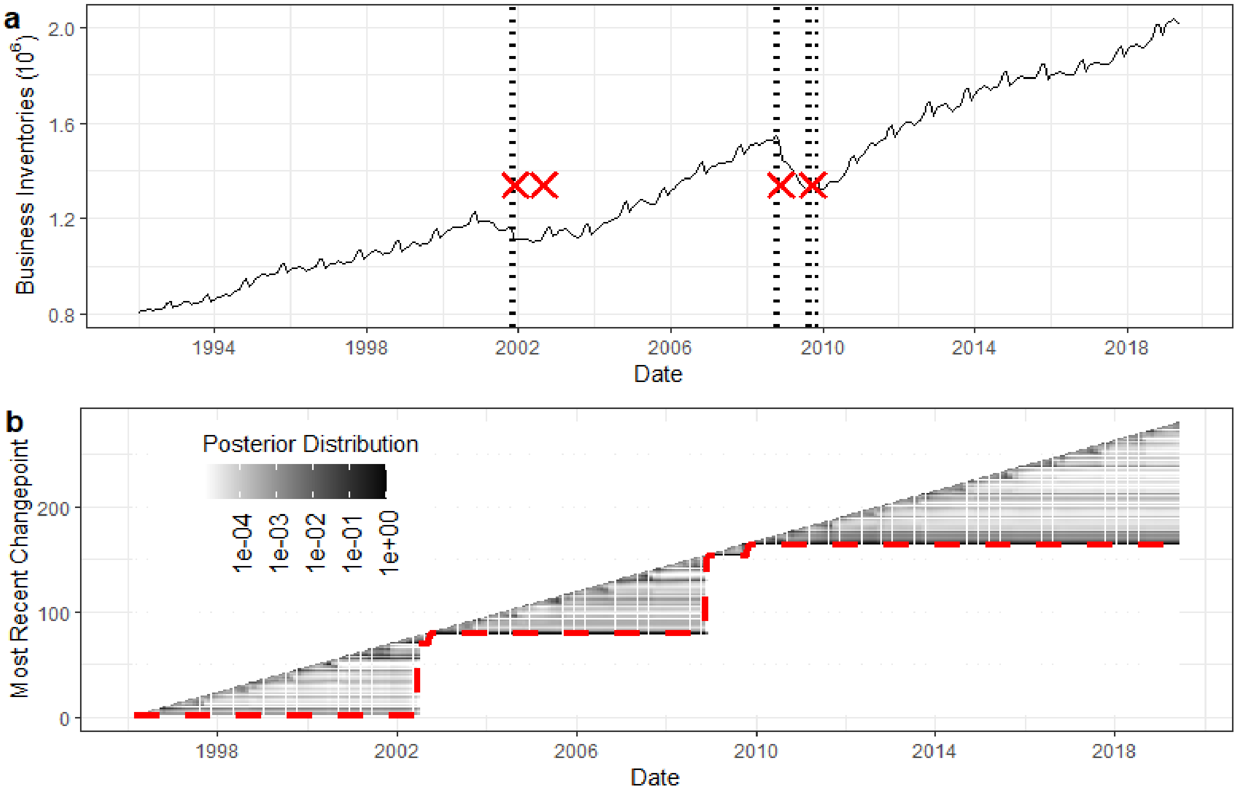


Figure S4: The outputs of SKF on the US monthly total business inventory data from 1992 to 2019. Panel a shows the monthly total business inventory data. The actual changepoints are marked by the black dashed lines. The estimated changepoints by SKF are marked by the red crossings. Panel b displays the posterior probability matrix of the most recent changepoints. The red dashed curve gives the estimated most recent changepoints with the maximum *a posterior* (MAP) estimator at each time step.

Box, G. E., G. M. Jenkins, G. C. Reinsel, and G. M. Ljung (2015). *Time series analysis: forecasting and control*. John Wiley & Sons.

Breiman, L. (2001). Random forests. *Machine learning 45*, 5–32.

Chen, T. and C. Guestrin (2016). XGBoost: A scalable tree boosting system. In *Proceedings of the 22nd acm sigkdd international conference on knowledge discovery and data mining*, pp. 785–794.

Duan, J., H. Li, X. Ma, H. Zhang, R. Lasky, C. K. Monaghan, S. Chaudhuri, L. A. Usvyat, M. Gu, W. Guo, P. Kotanko, and Y. Wang (2023). Predicting SARS-CoV-2 infection among hemodialysis patients using multimodal data. *Frontiers in Nephrology 3*, 1179342.

Fearnhead, P. and Z. Liu (2007). On-line inference for multiple changepoint problems. *Journal of the Royal Statistical Society: Series B (Statistical Methodology) 69*(4), 589–605.

Fearnhead, P. and Z. Liu (2011). Efficient Bayesian analysis of multiple changepoint models with dependence across segments. *Statistics and Computing 21*(2), 217–229.

Gu, M. and J. O. Berger (2016). Parallel partial Gaussian process emulation for computer models with massive output. *The Annals of Applied Statistics 10*(3), 1317–1347.

Gu, M. and Y. Xu (2020). Fast nonseparable Gaussian stochastic process with application to methylation level interpolation. *Journal of Computational and Graphical Statistics 29*(2), 250–260.

Gu, W., J. Choi, M. Gu, H. Simon, and K. Wu (2013). Fast change point detection for electricity market analysis. In *2013 IEEE International Conference on Big Data*, pp. 50–57. IEEE.

Hakki, S., J. Zhou, J. Jonnerby, A. Singanayagam, J. L. Barnett, K. J. Madon, A. Koycheva, C. Kelly, H. Houston, S. Nevin, J. Fenn, R. Kundu, M. A. Crone, T. D. Pillay, S. Ahmad, N. Derqui-Fernandez, E. Conibear, P. S. Freemont, G. P. Taylor, and N. Ferguson (2022). Onset and window of SARS-CoV-2 infectiousness and temporal correlation with symptom onset: a prospective, longitudinal, community cohort study. *The Lancet Respiratory Medicine 10*(11), 1061–1073.

Hartikainen, J. and S. Särkkä (2010). Kalman filtering and smoothing solutions to temporal Gaussian process regression models. In *2010 IEEE international workshop on machine learning for signal processing*, pp. 379–384. IEEE.

Jansen, L., B. Tegomoh, K. Lange, K. Showalter, J. Figliomeni, B. Abdalhamid, P. C. Iwen, J. Fauver, B. Buss, and M. Donahue (2021, 12). Investigation of a SARS-CoV-2 B.1.1.529 (Omicron) Variant Cluster — Nebraska, November–December 2021. *MMWR. Morbidity and Mortality Weekly Report 70*, 1782–1784.

Kurt, M. N., Y. Yılmaz, and X. Wang (2020). Real-time nonparametric anomaly detection in high-dimensional settings. *IEEE transactions on pattern analysis and machine intelligence 43*(7), 2463–2479.

Li, H. and M. Gu (2021). Robust estimation of SARS-CoV-2 epidemic in US counties. *Scientific reports 11*(1), 11841.

Monaghan, C. K., J. W. Larkin, S. Chaudhuri, H. Han, Y. Jiao, K. M. Bermudez, E. D. Weinhandl, I. A. Dahne-Steuber, K. Belmonte, L. Neri, P. Kotanko, J. P. Kooman, J. L. Hymes, R. J. Kossmann, L. A. Usvyat, and F. W. Maddux (2021). Machine learning for prediction of patients on hemodialysis with an undetected SARS-CoV-2 infection. *Kidney360 2*(3), 456.

Page, E. S. (1954). Continuous inspection schemes. *Biometrika 41*(1/2), 100–115.

Petris, G., S. Petrone, and P. Campagnoli (2009). Dynamic linear models. In *Dynamic linear models with R*, pp. 31–84. Springer.

Romano, G., G. Rigaill, V. Runge, and P. Fearnhead (2022). Detecting abrupt changes in the presence of local fluctuations and autocorrelated noise. *Journal of the American Statistical Association 117*(540), 2147–2162.

Saatçi, Y., R. D. Turner, and C. E. Rasmussen (2010). Gaussian process change point models. In *Proceedings of the 27th International Conference on Machine Learning (ICML-10)*, pp. 927–934.

Schölkopf, B. and A. J. Smola (2018). *Learning with Kernels: Support Vector Machines, Regularization, Optimization, and Beyond.* The MIT Press.

Song, J. S., J. Lee, M. Kim, H. S. Jeong, M. S. Kim, S. G. Kim, H. N. Yoo, J. J. Lee, H. Y. Lee, S.-E. Lee, E. J. Kim, J. E. Rhee, I. H. Kim, and Y.-J. Park (2022). Serial Intervals and Household Transmission of SARS-CoV-2 Omicron Variant, South Korea, 2021. *Emerging Infectious Diseases 28*, 756–759.

van den Burg, G. J. and C. K. Williams (2020). An evaluation of change point detection algorithms. *arXiv preprint arXiv:2003.06222*.
